# Supplementary material for: Automatic State Interaction with Large Localized Active Spaces for Multimetallic Systems
Source: arXiv:2403.15495 source file (2024-03-21)
Supplement: Supplementary file 3 [file 10_11.tex]

\begin{table}[]
\centering
\caption{Entropy for AlFeFe node with (11e,10o) active space for LASSI[1,5]. Fe$^{2+}$ in red and Fe$^{3+}$ in blue. $s_{K\mathcal{P}}$ is entropy for $K$th fragment in $\mathcal{P}$ rootspace. $q^\text{(avg)}$ is also provided for reference. 5 rootspaces are not shown due to low weights.}
\label{tab:my-table}
\begin{tabular}{c|>{\color{red}}c>{\color{blue}}c|>{\color{red}}c>{\color{blue}}c}
Rootspace  & \multicolumn{2}{c}{${s}_{\mathcal{P}K}$} & \multicolumn{2}{c}{$\bar{q}_{\mathcal{P}K}$} \\\hline
\multirow{5}{*}{\includegraphics[width=20mm]{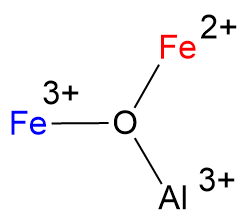}} 
& 0.00                & 0.00                & 0.00  & 0.00  \\
& 0.00                & 0.00                & 0.00  & 0.00  \\
& 0.00                & 0.00                & 0.00  & 0.00  \\
& 0.00                & 0.00                & 0.00  & 0.00  \\
& 0.00                & 0.00                & 0.00  & 0.00  \\\hline
\multirow{5}{*}{\includegraphics[width=20mm]{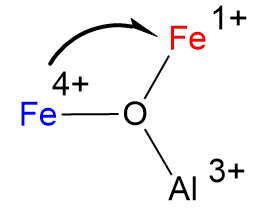}} 
& 0.77                & 0.77                & 0.87  & 1.87  \\
& 0.79                & 0.79                & 0.95  & 1.87  \\
& 0.79                & 0.79                & 0.99  & 1.87  \\
& 0.79                & 0.79                & 0.91  & 1.87  \\
&&&&\\\hline
\multirow{5}{*}{\includegraphics[width=20mm]{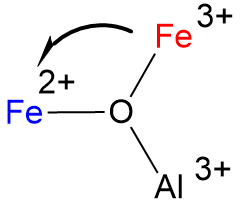}} 
& 1.03                & 1.03                & 1.20  & 1.11  \\
& 1.02                & 1.02                & 1.21  & 1.11  \\
& 1.02                & 1.02                & 1.21  & 1.12  \\
& 1.02                & 1.02                & 1.21  & 1.10  \\
&&&&\\\hline
\end{tabular}
\end{table}
