# Supplementary material for: Automatic State Interaction with Large Localized Active Spaces for Multimetallic Systems
Source: arXiv:2403.15495 source file (2024-03-21)
Supplement: Supplementary file 4 [file 20_11.tex]

\begin{table}[]
\centering
\caption{Entropy for AlFeFe node with (11e,20o) active space with LASSI[1,15]. Fe$^{2+}$ in red and Fe$^{3+}$ in blue. $s_{K\mathcal{P}}$ is entropy for $K$th fragment in $\mathcal{P}$ rootspace. $q^\text{(avg)}$ is also provided for reference. Note that even though $n^\text{(avg)}$ can be really high, the entropy is close to 1. \textcolor{red}{updated}}
\label{tab:20_11_entropy}
\begin{tabular}{c|>{\color{red}}c>{\color{blue}}c|>{\color{red}}c>{\color{blue}}c}
Rootspace  & \multicolumn{2}{c}{${s}_{\mathcal{P}K}$} & \multicolumn{2}{c}{$\bar{q}_{\mathcal{P}K}$} \\\hline
\multirow{9}{*}{\includegraphics[width=20mm]{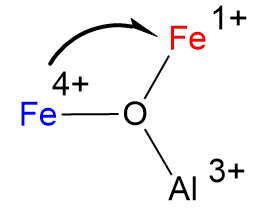}}
& 0.14 & 0.14 & 2.27 & 1.68 \\
& 0.82 & 0.82 & 2.09 & 2.14 \\
& 0.14 & 0.14 & 2.27 & 1.70 \\
& 0.82 & 0.82 & 2.10 & 2.14 \\
& 0.14 & 0.14 & 2.27 & 1.73 \\
& 0.82 & 0.82 & 2.10 & 2.15 \\
& 0.22 & 0.16 & 2.30 & 1.70 \\
& 0.14 & 0.14 & 2.27 & 1.72 \\
& 0.82 & 0.82 & 2.10 & 2.14 \\\hline
\multirow{5}{*}{\includegraphics[width=20mm]{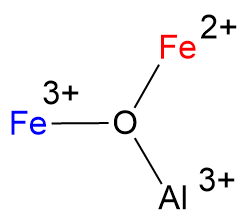}}
&0.00 & 0.00 & 0.00 & 0.00 \\
&0.00 & 0.00 & 0.00 & 0.00 \\
&0.00 & 0.00 & 0.00 & 0.00 \\
&0.00 & 0.00 & 0.00 & 0.00 \\
&0.00 & 0.00 & 0.00 & 0.00 \\\hline
\multirow{19}{*}{\includegraphics[width=20mm]{Figures/SI/DiIron/f-1f1.png}}&0.13 & 0.13 & 0.16 & 2.69 \\
& 0.13 & 0.13 & 0.16 & 2.69 \\
& 0.22 & 0.34 & 6.98 & 1.86 \\
& 0.00 & 0.00 & 0.02 & 1.83 \\
& 0.13 & 0.13 & 0.16 & 2.69 \\
& 1.01 & 0.92 & 5.66 & 1.20 \\
& 0.20 & 0.21 & 7.01 & 2.09 \\
& 0.00 & 0.06 & 0.02 & 1.72 \\
& 0.13 & 0.13 & 0.16 & 2.69 \\
& 0.00 & 0.00 & 0.02 & 1.75 \\
& 0.22 & 0.25 & 6.98 & 2.24 \\
& 1.01 & 0.92 & 5.69 & 1.20 \\
& 0.13 & 0.13 & 0.16 & 2.69 \\
& 0.00 & 0.00 & 0.02 & 1.80 \\
& 0.24 & 0.37 & 6.88 & 2.28 \\
& 0.98 & 0.91 & 5.57 & 1.18 \\
& 0.13 & 0.13 & 0.16 & 2.69 \\
& 1.06 & 0.93 & 5.74 & 1.21 \\
& 0.13 & 0.13 & 0.16 & 2.69 \\\hline
\end{tabular}
\end{table}
