# Supplementary material for: Automatic State Interaction with Large Localized Active Spaces for Multimetallic Systems
Source: arXiv:2403.15495 source file (2024-03-21)
Supplement: Supplementary file 6 [file 15_16_table.tex]

\begin{table*}[]
\centering
\caption{Absolute energies for LASSI and LAS-CASCI upto 6 decimal digits in Fe$_3$ system with (16e,15o) active space.}
\label{tab:15_16_energies}
\begin{tabular}{|c|c|c|c|c|c|}
\hline
Spin   & LASSI[0,1]   & LASSI[1,1]   & LASSI[1,5]   & LASSI[1,5$_\text{CT}$] & LAS-CASCI    \\\hline
S=7 & -4992.234449 & -4992.234449 & -4992.234449 & -4992.234449 & -4992.234449 \\
S=6 & -4992.233872 & -4992.234049 & -4992.235012 & -4992.235012 & -4992.235015 \\
S=5 & -4992.233378 & -4992.233695 & -4992.235479 & -4992.235479 & -4992.235489 \\
S=4 & -4992.232966 & -4992.233392 & -4992.235854 & -4992.235854 & -4992.235871 \\
S=3 & -4992.232637 & -4992.233143 & -4992.236140 & -4992.236140 & -4992.236165 \\
S=2 & -4992.232127 & -4992.232597 & -4992.236344 & -4992.236344 & -4992.236376 \\
S=1 & -4992.231751 & -4992.232181 & -4992.236360 & -4992.236360 & -4992.236394 \\
S=0 & -4992.231511 & -4992.231869 & -4992.236311 & -4992.236311 & -4992.236345 \\\hline
States & 24           & 182          & 6910         & 3014          &  41.4 million           \\\hline
\end{tabular}
\end{table*}
