# Supplementary material for: Automatic State Interaction with Large Localized Active Spaces for Multimetallic Systems
Source: arXiv:2403.15495 source file (2024-03-21)
Supplement: Supplementary file 7 [file 30_16_table.tex]

\begin{table*}[]
\centering
\caption{}
\label{tab:my-table}
\caption{(Absolute energies + 4992.36 $E_h$)$\times 100$ for LASSI and LAS-DMRGCI upto 6 decimal digits in Fe$_3$ system with (16e,30o) active space.}
\label{tab:30_16_energies}
\begin{tabular}{|c|c|c|c|c|c|c|c|c|c|}
\hline
&\multicolumn{8}{c|}{LASSI}&\\\hline
Spin   & [0,1] & [1,1] &  [1,3$_\text{CT}$] & [1,4$_\text{CT}$] & [1,5$_\text{CT}$] & [1,6$_\text{CT}$] & [1,7$_\text{CT}$] & [1,8$_\text{CT}$] & DMRGCI \\\hline
7      & -0.5901  & -0.5942  & -0.5964 & -0.6269 & -0.6271 & -0.6287 & -0.6289 & -0.6290 & -0.6985 \\
6      & -0.5324  & -0.5382  & -0.5782 & -0.6841 & -0.6938 & -0.6965 & -0.6970 & -0.7001 & -0.7835 \\
5      & -0.4830  & -0.4901  & -0.5623 & -0.7300 & -0.7472 & -0.7509 & -0.7518 & -0.7580 & -0.8544 \\
4      & -0.4418  & -0.4500  & -0.5488 & -0.7648 & -0.7877 & -0.7924 & -0.7937 & -0.8031 & -0.9114 \\
3      & -0.4088  & -0.4178  & -0.5378 & -0.7893 & -0.8159 & -0.8219 & -0.8234 & -0.8363 & -0.9552 \\
2      & -0.3596  & -0.3712  & -0.5295 & -0.8050 & -0.8334 & -0.8408 & -0.8427 & -0.8591 & -0.9868 \\
1      & -0.3235  & -0.3167  & -0.5196 & -0.7846 & -0.8166 & -0.8245 & -0.8269 & -0.8453 & -0.9906 \\
0      & -0.3006  & -0.3088  & -0.5133 & -0.7597 & -0.7917 & -0.8007 & -0.8036 & -0.8246 & -0.9846 \\\hline
States & 24         & 380        & 3228      & 5720      & 8924      & 12840     & 17468     & 22808     &34 Trillion \\\hline             
\end{tabular}
\end{table*}
