# Supplementary material for: Automatic State Interaction with Large Localized Active Spaces for Multimetallic Systems
Source: arXiv:2403.15495 source file (2024-03-21)
Supplement: Supplementary file 9 [file n_variation_plot.tex]

\begin{table}
%\adjustbox{max width=\columnwidth}{...}
\begin{tabular}[c]{|c|c|c|ccccc|c|}
%\label{tab:alfe2-full}\\\hline
%AS              & 1,$n^\text{(max)}$ & States & S=9/2        & S=7/2        & S=5/2        & S=3/2        & S=1/2        & J     \\\hline
%\endfirsthead
%
%\multicolumn{9}{c}%
%{{\bfseries Table \thetable\ continued from previous page}} \\
AS               & LASSI[1,$q$]& States & S=9/2        & S=7/2        & S=5/2        & S=3/2        & S=1/2        & J      \\\hline
%\endhead
%
\multirow{6}{*}{(11,10)}&q=1& 18    & -0.792354 & -0.787674 & -0.783994 & -0.781369 & -0.77982 & 114.65 \\
 &q=2& 52    & -0.792354 & -0.788224 & -0.785009 & -0.782712 & -0.781336 & 100.75 \\
 &q=3& 102   & -0.792354 & -0.790834 & -0.789668 & -0.788841 & -0.788318 & 36.91  \\
 &q=4& 168   & -0.792354 & -0.792213 & -0.792078 & -0.791969 & -0.791898 & 4.17   \\
 &q=5& 250   & -0.792354 & -0.792507 & -0.792598 & -0.792647 & -0.792671 & -2.90  \\
 &\multicolumn{8}{c|}{$q=6$ to $q=10$ are same as $q=5$ upto 6 decimal points.}\\\cline{2-9}
 %&q=6& 290   & -0.792354 & -0.792507 & -0.792598 & -0.792647 & -0.792671 & -2.90  \\
 %&q=7& 330   & -0.792354 & -0.792507 & -0.792598 & -0.792647 & -0.792671 & -2.90  \\
 %&q=8& 370   & -0.792354 & -0.792507 & -0.792598 & -0.792647 & -0.792671 & -2.90  \\
 %&q=9& 410   & -0.792354 & -0.792507 & -0.792598 & -0.792647 & -0.792671 & -2.90  \\
 %&q=10& 450   & -0.792354 & -0.792507 & -0.792598 & -0.792647 & -0.792671 & -2.90  \\\cline{2-9}
 & CASCI         & 52920  &-0.792354 & -0.792511  & -0.792632 &              & -0.792771 & -3.81\\ \hline
\multirow{11}{*}{(9,9)} &q=1 & 13 & -0.792354 & -0.787678 & -0.7839990 & -0.7813737 & -0.779823 & 114.60 \\
&q=2  & 29  & -0.792354 & -0.788227 & -0.7850137 & -0.782718 & -0.781344 & 100.69 \\
&q=3  & 37  & -0.792354 & -0.790845 & -0.7896879 & -0.788868 & -0.788348 & 36.64  \\
&q=4  & 77 & -0.792354 & -0.792214 & -0.7920803 & -0.791972 & -0.791902 & 4.14   \\
&q=5  & 133 & -0.792354 & -0.792507 & -0.7925973 & -0.792646 & -0.792670 & -2.89  \\
% &\multicolumn{8}{c|}{$q=6$ to $q=10$ are same as $q=5$ upto 6 decimal points.}\\\hline
&q=6  & 165 & -0.792354 & -0.792507 & -0.792597 & -0.792646 & -0.792670 & -2.89  \\
&q=7  & 165 & -0.792354 & -0.792507 & -0.792597 & -0.792646 & -0.792670 & -2.89  \\
&q=8  & 165 & -0.792354 & -0.792507 & -0.792597 & -0.792646 & -0.792670 & -2.89  \\
&q=9  & 165 & -0.792354 & -0.792507 & -0.792597 & -0.792646 & -0.792670 & -2.89  \\
&q=10 & 165 & -0.792354 & -0.792507 & -0.792597 & -0.792646 & -0.792670 & -2.89  \\\cline{2-9}
& CASCI & 15876  & -0.792354 & -0.792511 & -0.792632 &              & -0.792770 & -3.81  \\\hline
\multirow{12}{*}{(11,20)} & q=1  & 33    & -0.891148 & -0.890886 & -0.890684 & -0.890539 & -0.890451 & 6.37  \\
&q=3  & 297   & -0.891157 & -0.890960 & -0.890808 & -0.890700 & -0.890632 & 4.80  \\
&q=5  & 825   & -0.891299 & -0.891212 & -0.891151 & -0.891111 & -0.891087 & 1.94  \\
&q=7  & 1617  & -0.891311 & -0.891239 & -0.891191 & -0.891161 & -0.891141 & 1.56  \\
&q=9  & 2673  & -0.891311 & -0.891299 & -0.891296 & -0.891297 & -0.891301 & 0.10  \\
&q=11 & 3993  & -0.891318 & -0.891320 & -0.891329 & -0.891338 & -0.891347 & -0.27 \\
&q=13 & 5577  & -0.891318 & -0.891389 & -0.891453 & -0.891503 & -0.891533 & -1.97 \\
&q=15 & 7425  & -0.891318 & -0.891462 & -0.891580 & -0.891666 & -0.891720 & -3.67 \\
&q=17 & 9537  & -0.891319 & -0.891467 & -0.891588 & -0.891678 & -0.891732 & -3.78 \\
&q=19 & 11913 & -0.891468 & -0.891468 & -0.891589 & -0.891678 & -0.891733 & -2.43 \\
&q=21 & 14553 & -0.891333 & -0.891528 & -0.891684 & -0.891799 & -0.891868 & -4.89\\\cline{2-9}
& CASCI& $6 \times 10^8$ &-0.891595 & -0.891848 &-0.892047 & -0.892191 &    -0.892278 & -6.245\\ \hline
\end{tabular}
\caption{Absolute energies + 3971 $E_h$ for various LASSI[$r=1$, $q$] and $J$ with AlFe$_2$ for (11e,10o), (9e,9o) and (11e,20o) active spaces. Note that (9e,9o) and (11e,10o) results are nearly identical, suggesting that the doubly occupied orbital is not contributing to the magnetic exchange coupling interaction.}
\end{table}
