# Supplementary material for: Automatic State Interaction with Large Localized Active Spaces for Multimetallic Systems
Source: arXiv:2403.15495 source file (2024-03-21)
Supplement: Supplementary file 10 [file AlFeFe.tex]

\begin{table}[]
\centering
\caption{Geometry of Al-Fe-Fe MOF Node. All values in $\AA$}
\label{tab:my-table}

\begin{tabular}{cccc}
O  & -2.220198244  & 0.3991903003  & 1.694471699   \\
O  & -1.685553245  & -1.782306322  & 1.431399507   \\
C  & -2.268517865  & -0.8319550379 & 1.983951274   \\
H  & -2.913342017  & -1.076728589  & 2.843786805   \\
O  & 1.388288081   & 2.079556156   & -1.347085675  \\
O  & -0.7599088595 & 2.580923635   & -0.849227704  \\
C  & 0.3465674686  & 2.753895325   & -1.438835699  \\
H  & 0.3723796145  & 3.61769966    & -2.12309115   \\
O  & 1.046960908   & -2.6425342    & 0.9613246722  \\
O  & -0.3991903003 & 2.220198244   & 1.694471699   \\
O  & 1.782306322   & 1.685553245   & 1.431399507   \\
C  & 0.8319550379  & 2.268517865   & 1.983951274   \\
H  & 1.076728589   & 2.913342017   & 2.843786805   \\
O  & -2.079556156  & -1.388288081  & -1.347085675  \\
O  & -2.580923635  & 0.7599088595  & -0.849227704  \\
C  & -2.753895325  & -0.3465674686 & -1.438835699  \\
H  & -3.61769966   & -0.3723796145 & -2.12309115   \\
Fe & -0.3798741893 & -1.792603363  & -0.2003377303 \\
O  & 0.6422231803  & -2.237796553  & -1.892914518  \\
Fe & 1.792603363   & 0.3798741893  & -0.2003377303 \\
O  & 2.237796553   & -0.6422231803 & -1.892914518  \\
O  & 2.6425342     & -1.046960908  & 0.9613246722  \\
Al & -1.236271642  & 1.236271642   & 0.350650148   \\
O  & -0.0449501954 & 0.0449501954  & 0.0127621413  \\
C  & 1.645528685   & -1.645528685  & -2.357112465  \\
H  & 2.056906298   & -2.056906298  & -3.294571292  \\
C  & 2.160924281   & -2.160924281  & 1.277584187   \\
H  & 2.796080543   & -2.796080543  & 1.918244302  
\end{tabular}
\end{table}
