# Supplementary material for: Automatic State Interaction with Large Localized Active Spaces for Multimetallic Systems
Source: arXiv:2403.15495 source file (2024-03-21)
Supplement: Supplementary file 11 [file FeFeFe.tex]

\begin{table}[]
\centering
\caption{Geometry of Fe-Fe-Fe MOF Node. All values in $\AA$}
\label{tab:Fe3_Geom}
\begin{tabular}{cccc}
O  & -1.396530536  & -2.155053668  & 1.497463409  \\
O  & -1.424929948  & -0.1579202181 & 2.556757216  \\
C  & -1.805663158  & -1.333357733  & 2.354770591  \\
H  & -2.611139824  & -1.698287377  & 3.015172572  \\
O  & 1.422169433   & -0.1727766066 & -2.448307975 \\
O  & 1.404243292   & -2.165442677  & -1.387375376 \\
C  & 1.812327533   & -1.345288486  & -2.246529164 \\
H  & 2.621336914   & -1.706173551  & -2.904090708 \\
O  & -1.428899418  & 2.343625706   & 1.186473538  \\
O  & -1.403562858  & -2.165307125  & -1.387572278 \\
O  & -1.422998602  & -0.1723629226 & -2.447964967 \\
C  & -1.812500488  & -1.345105901  & -2.246279414 \\
H  & -2.621699381  & -1.706195274  & -2.903496624 \\
O  & 1.425112371   & -0.1571948062 & 2.556693752  \\
O  & 1.397382095   & -2.154305543  & 1.497360669  \\
C  & 1.806221904   & -1.332524996  & 2.35469992   \\
H  & 2.611813123   & -1.697184248  & 3.015110605  \\
Fe & -0.0001429864 & 0.9716426461  & 1.624782043  \\
O  & 1.428198549   & 2.344050002   & 1.186026051  \\
Fe & -0.0001364224 & 0.952927878   & -1.522872889 \\
O  & 1.423595107   & 2.330128125   & -1.070103354 \\
O  & -1.423503945  & 2.330456754   & -1.069656998 \\
Fe & 0.0002549988  & -1.941619777  & 0.0458885284 \\
O  & -0.0001521382 & -0.0719149875 & 0.0721478962 \\
C  & 1.815220274   & 2.721515148   & 0.0544222441 \\
H  & 2.604057215   & 3.492625269   & 0.0488314748 \\
C  & -1.815568952  & 2.721425035   & 0.0548464944 \\
H  & -2.604489027  & 3.492449072   & 0.0492507598
\end{tabular}
\end{table}
